# Supplementary material for: Arithmetic of quaternion origami
Source: arXiv:1805.04046 source file (2018-05-10)
Supplement: Supplementary file 1 [file appendixB.tex]

\begin{center} \textbf{Appendix B} \end{center}

The map $k_g \rightarrow k_1$ given by $\alpha \mapsto \beta = \frac{-1}{3^2b}(\alpha^3-4a\alpha^2+(8a^2-72bz)\alpha +2^4 3 d)$ is an isomorphism, where $\alpha$ is a root of $g$. In this appendix, we show that $\beta$ satisfies the defining polynomial $h_1$ of $k_1$.

\begin{equation*}
\begin{split}
3^8b^4h_1(\beta) &= \alpha^{12} - 2^4a\alpha^{11} + (2^55a^2 - 2^53^2bz)\alpha^{10} + (-2^8a^3 + 2^73^3abz + 2^63^4b^2)\alpha^9 \\
& + (-2^817a^4 - 2^{10}3^3a^2bz 
- 2^83^5ab^2 + 2^73^5b^2z^2)\alpha^8 \\
&+ (2^{13}7a^5 -2^{12}3^2a^3bz + 2^{11}3^5a^2b^2 - 2^{10}3^5ab^2z^2 - 
    2^93^7b^3z)\alpha^7  \\
    &+ (-2^{14}5a^6 + 2^{15}3^3a^4bz + 2^{11}3^5a^3b^2 + 2^{11}3^6a^2b^2z^2 + 2^{12}3^7ab^3z + 
    2^{12}3^7b^4 - 2^{11}3^6b^3z^3)\alpha^6 \\
    &+ (-2^{17}5a^7 - 2^{18}3^3a^5bz - 2^{14}3^411a^4b^2 + 2^{15}3^5a^3b^2z^2 
    - 2^{13}3^8a^2b^3z - 2^{15}3^7ab^4 +\\
    &  2^{13}3^6ab^3z^3    + 2^{12}3^9b^4z^2)\alpha^5 + (2^{16}127a^8 - 2^{18}3^25a^6bz
    + 2^{15}3^65a^5b^2 - 2^{15}3^55a^4b^2z^2 -\\
    &  2^{15}3^611a^3b^3z + 2^{16}3^8a^2b^4 - 2^{15}3^6a^2b^3z^3 - 
    2^{14}3^9ab^4z^2 - 2^{16}3^9b^5z + 2^{12}3^8b^4z^4)\alpha^4 \\
    & + (2^{20}3a^9  + 2^{20}3^4a^7bz + 
    2^{21}3^4a^6b^2 + 2^{18}3^6a^5b^2z^2 + 2^{18}3^67a^4b^3z + 2^{16}3^713a^3b^4\\
    &  - 2^{17}3^7a^3b^3z^3 
     - 2^{17}3^6a^3b^3w^2 + 2^{16}3^9a^2b^4z^2 + 2^{18}3^9ab^5z + 2^{15}3^{11}b^6 - 2^{15}3^{10}b^5z^3 \\
    &- 2^{15}3^9b^5w^2)\alpha^3 + (-2^{21}3^3a^{10} - 2^{21}3^5a^8bz - 2^{19}3^431a^7b^2 + 2^{19}3^7a^6b^2z^2\\
    & - 2^{19}3^617a^5b^3z - 2^{18}3^717a^4b^4 + 2^{19}3^6a^4b^3w^2 + 2^{17}3^817a^3b^4z^2 - 
    2^{20}3^9a^2b^5z \\
    &- 2^{17}3^{11}ab^6 + 2^{17}3^9ab^5w^2 + 2^{18}3^{11}b^6z^2)\alpha^2 + 
     (2^{24}3^3a^{11} - 2^{23}3^5a^9bz +\\
     & 2^{25}3^5a^8b^2 - 2^{24}3^7a^6b^3z + 2^{20}3^87a^5b^4 - 2^{21}3^6a^5b^3w^2 - 
    2^{19}3^{10}7a^3b^5z + \\
    & 2^{20}3^8a^3b^4zw^2 + 2^{19}3^{11}a^2b^6 - 2^{19}3^9a^2b^5w^2 - 
    2^{18}3^{13}b^7z + 2^{18}3^{11}b^6zw^2)\alpha \\
    & + 2^{24}3^4a^{12} + 2^{23}3^65a^9b^2 + 2^{22}3^{10}a^6b^4 - 
    2^{23}3^7a^6b^3w^2 -2^{20}3^{10}a^5b^4z^2  \\
    & + 2^{20}3^9a^4b^4zw^2 +2^{18}3^{11}19a^3b^6 + 
    2^{20}3^{11}a^3b^5z^3 - 2^{20}3^{10}5a^3b^5w^2 \\
    &- 2^{18}3^{13}a^2b^6z^2 + 2^{18}3^{12}ab^6zw^2 + 
    2^{18}3^{14}b^8 + 2^{18}3^{14}b^7z^3 - 2^{18}3^{14}b^7w^2
\end{split}
\end{equation*}

    After, reducing using that $\alpha^4=
4\Delta \alpha+12 a \Delta$, this polynomial can be written as $c_3 \alpha^3+c_2\alpha^2+c_1 \alpha+c_0$ where the coefficients are the following:

$c_3= 2^{17}3^6a^4b^3z + 2^{17}3^6a^3b^4 + 2^{17}3^6a^3b^3z^3 - 2^{17}3^6a^3b^3w^2 + 2^{15}3^9ab^5z + 2^{15}3^9b^6 + 2^{15}3^9b^5z^3 - 2^{15}3^9b^5w^2$\\
 
$c_2=-2^{19}3^6a^5b^3z - 2^{19}3^6a^4b^4 - 2^{19}3^6a^4b^3z^3 + 2^{19}3^6a^4b^3w^2 - 2^{17}3^9a^2b^5z - 2^{17}3^9ab^6 - 2^{17}3^9ab^5z^3 + 2^{17}3^9ab^5w^2$\\
 
 $c_1=2^{21}3^6a^6b^3z + 2^{21}3^6a^5b^4 + 2^{21}3^6a^5b^3z^3 - 
    2^{21}3^6a^5b^3w^2 - 2^{20}3^8a^4b^4z^2 + 2^{19}3^8a^3b^5z - 2^{20}3^8a^3b^4z^4 + 
    2^{20}3^8a^3b^4zw^2 + 2^{19}3^9a^2b^6 + 2^{19}3^9a^2b^5z^3 - 2^{19}3^9a^2b^5w^2 - 2^{18}3^{11}ab^6z^2 - 2^{18}3^{11}b^7z - 2^{18}3^{11}b^6z^4 + 2^{18}3^{11}b^6zw^2$\\
    
 $c_0=2^{23}3^7a^7b^3z + 2^{23}3^7a^6b^4 + 2^{23}3^7a^6b^3z^3 - 2^{23}3^7a^6b^3w^2 -  2^{20}3^9a^5b^4z^2 + 2^{21}3^97a^4b^5z - 2^{20}3^9a^4b^4z^4 + 2^{20}3^9a^4b^4zw^2 +   2^{20}3^{10}5a^3b^6 +  2^{20}3^{10}5a^3b^5z^3 - 2^{20}3^{10}5a^3b^5w^2 - 2^{18}3^{12}a^2b^6z^2 + 2^{21}3^{12}ab^7z - 2^{18}3^{12}ab^6z^4 + 2^{18}3^{12}ab^6zw^2 + 2^{18}3^{14}b^8 + 2^{18}3^{14}b^7z^3 - 2^{18}3^{14}b^7w^2$
